# Supplementary material for: TRAM: Global Trajectory and Motion of 3D Humans from in-the-wild Videos
Source: arXiv:2403.17346 source file (2024-09-02)
Supplement: Supplementary file 1 [file supp_a.tex]

\section{Additional Experiments}

\subsection{Naive Combination: DROID + ZoeDepth}

\begin{figure*}[ht!]
\vspace{-6mm}
\centering
   \includegraphics[width=1.0\textwidth]{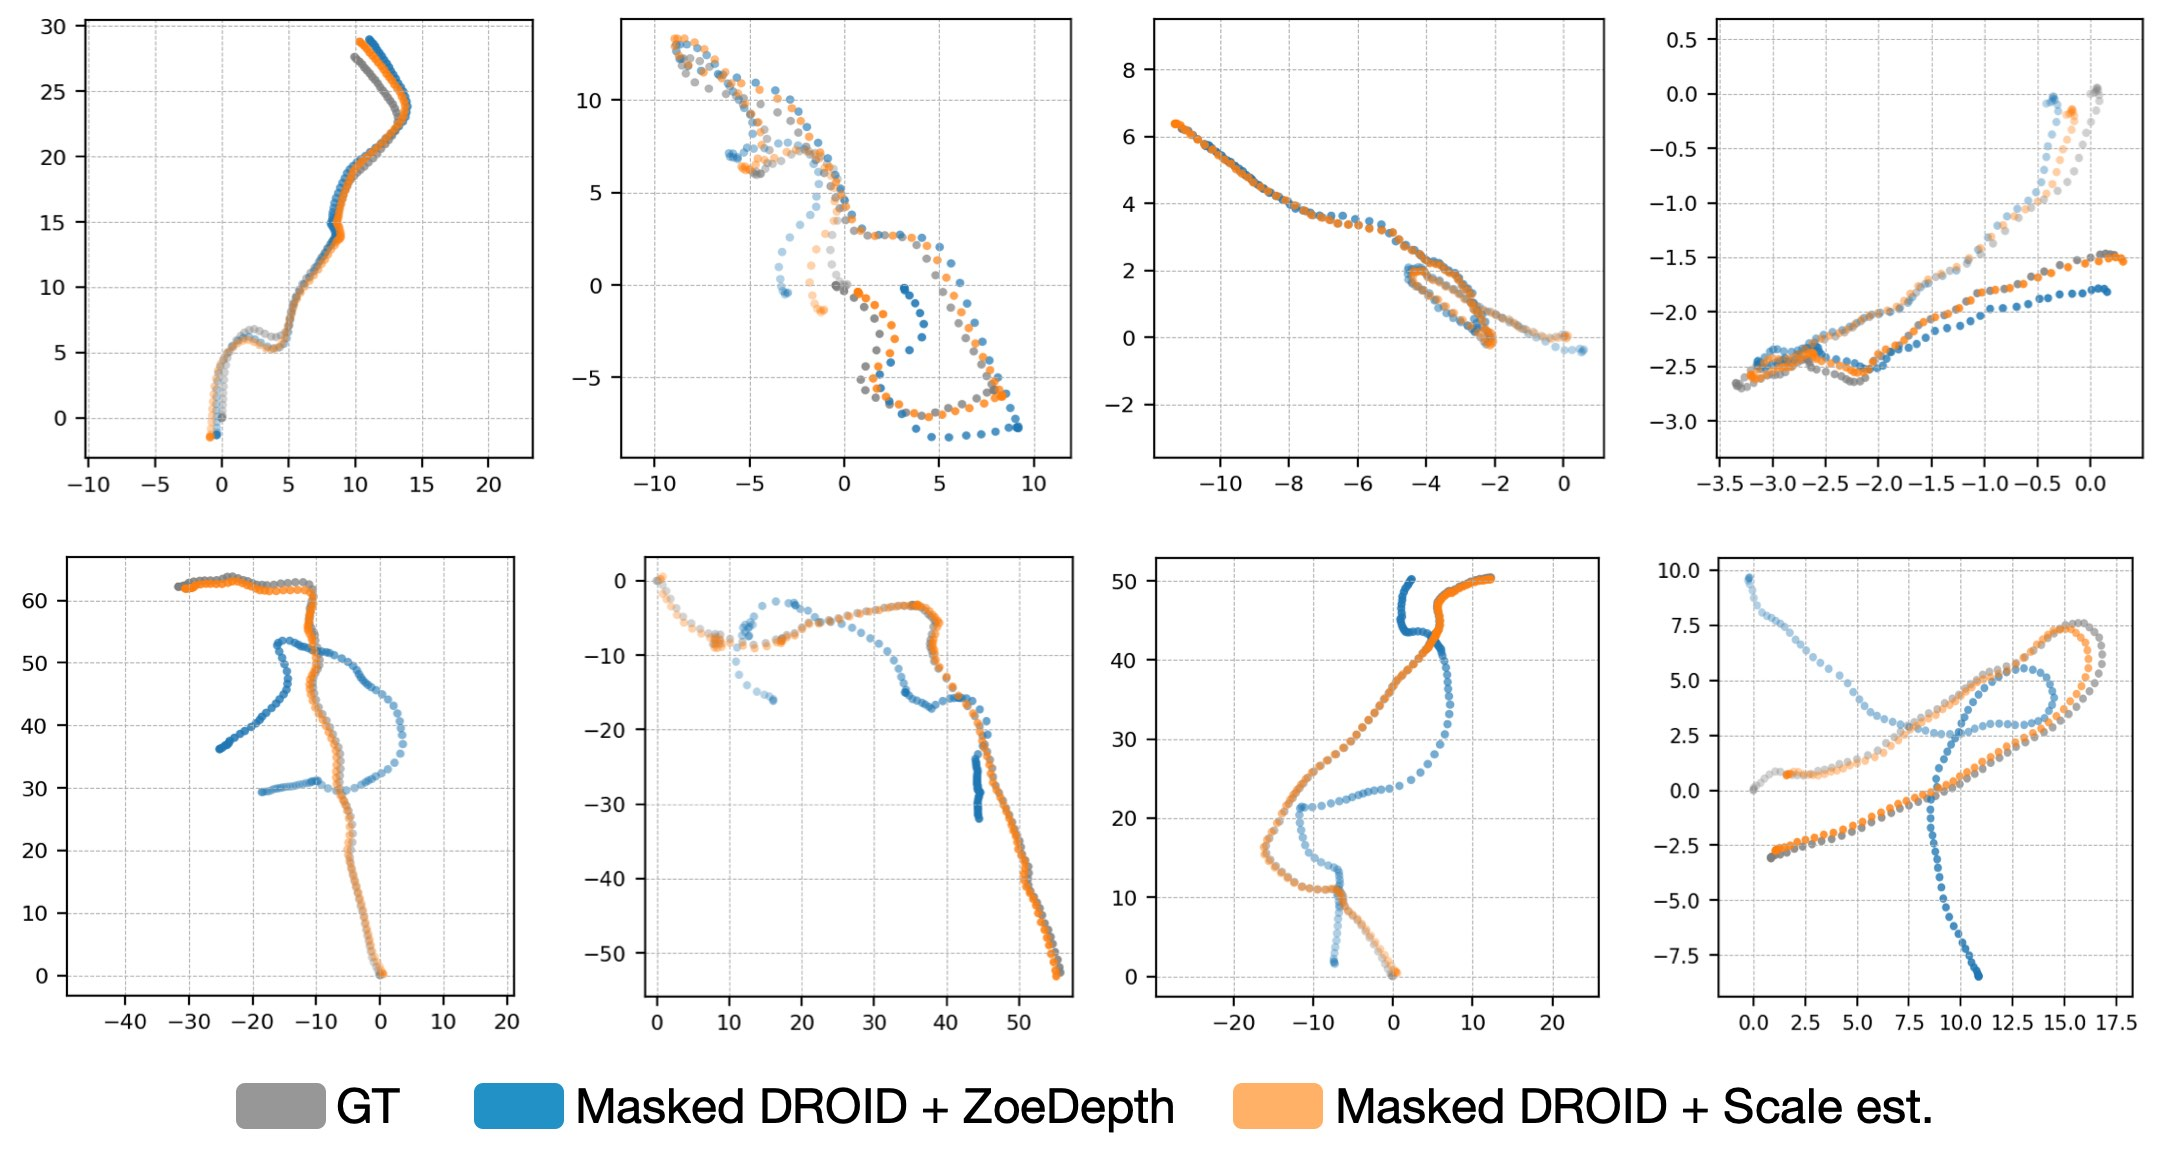}
   \vspace{-6mm}
    \caption{\textbf{Camera trajectory.} Top row: examples where the naive combination achieves comparable results. Bottom row: naive combination leads to large error. }
    \vspace{-3mm}
    \label{fig:cam_traj_zoe}
\end{figure*}

Our method TRAM derives camera motion scale from the background, by using a robust optimization procedure to align SLAM depth with predicted metric depth (Sec~\ref{sec:3_3}). As an alternative, we could give metric depth prediction to SLAM along with the input images as pseudo RGB-D inputs. RGB-D SLAM will then return trajectory in metric scale. As indicated in the main text, this naive approach leads to an average ATE-S of 3.09$m$, while our method has an average ATE-S of 0.66$m$. We visualize this difference in Figure~\ref{fig:cam_traj_zoe}. As shown, DROID diverges in roughly half of the sequences due to noisy or spurious depth predictions. Metric depth prediction cannot be treated as RGB-D inputs for a SLAM system. 
\clearpage

\subsection{Using SMPL Depth to Improve ZoeDepth}

\begin{figure*}[t!]
\centering
   \includegraphics[width=0.8\textwidth]{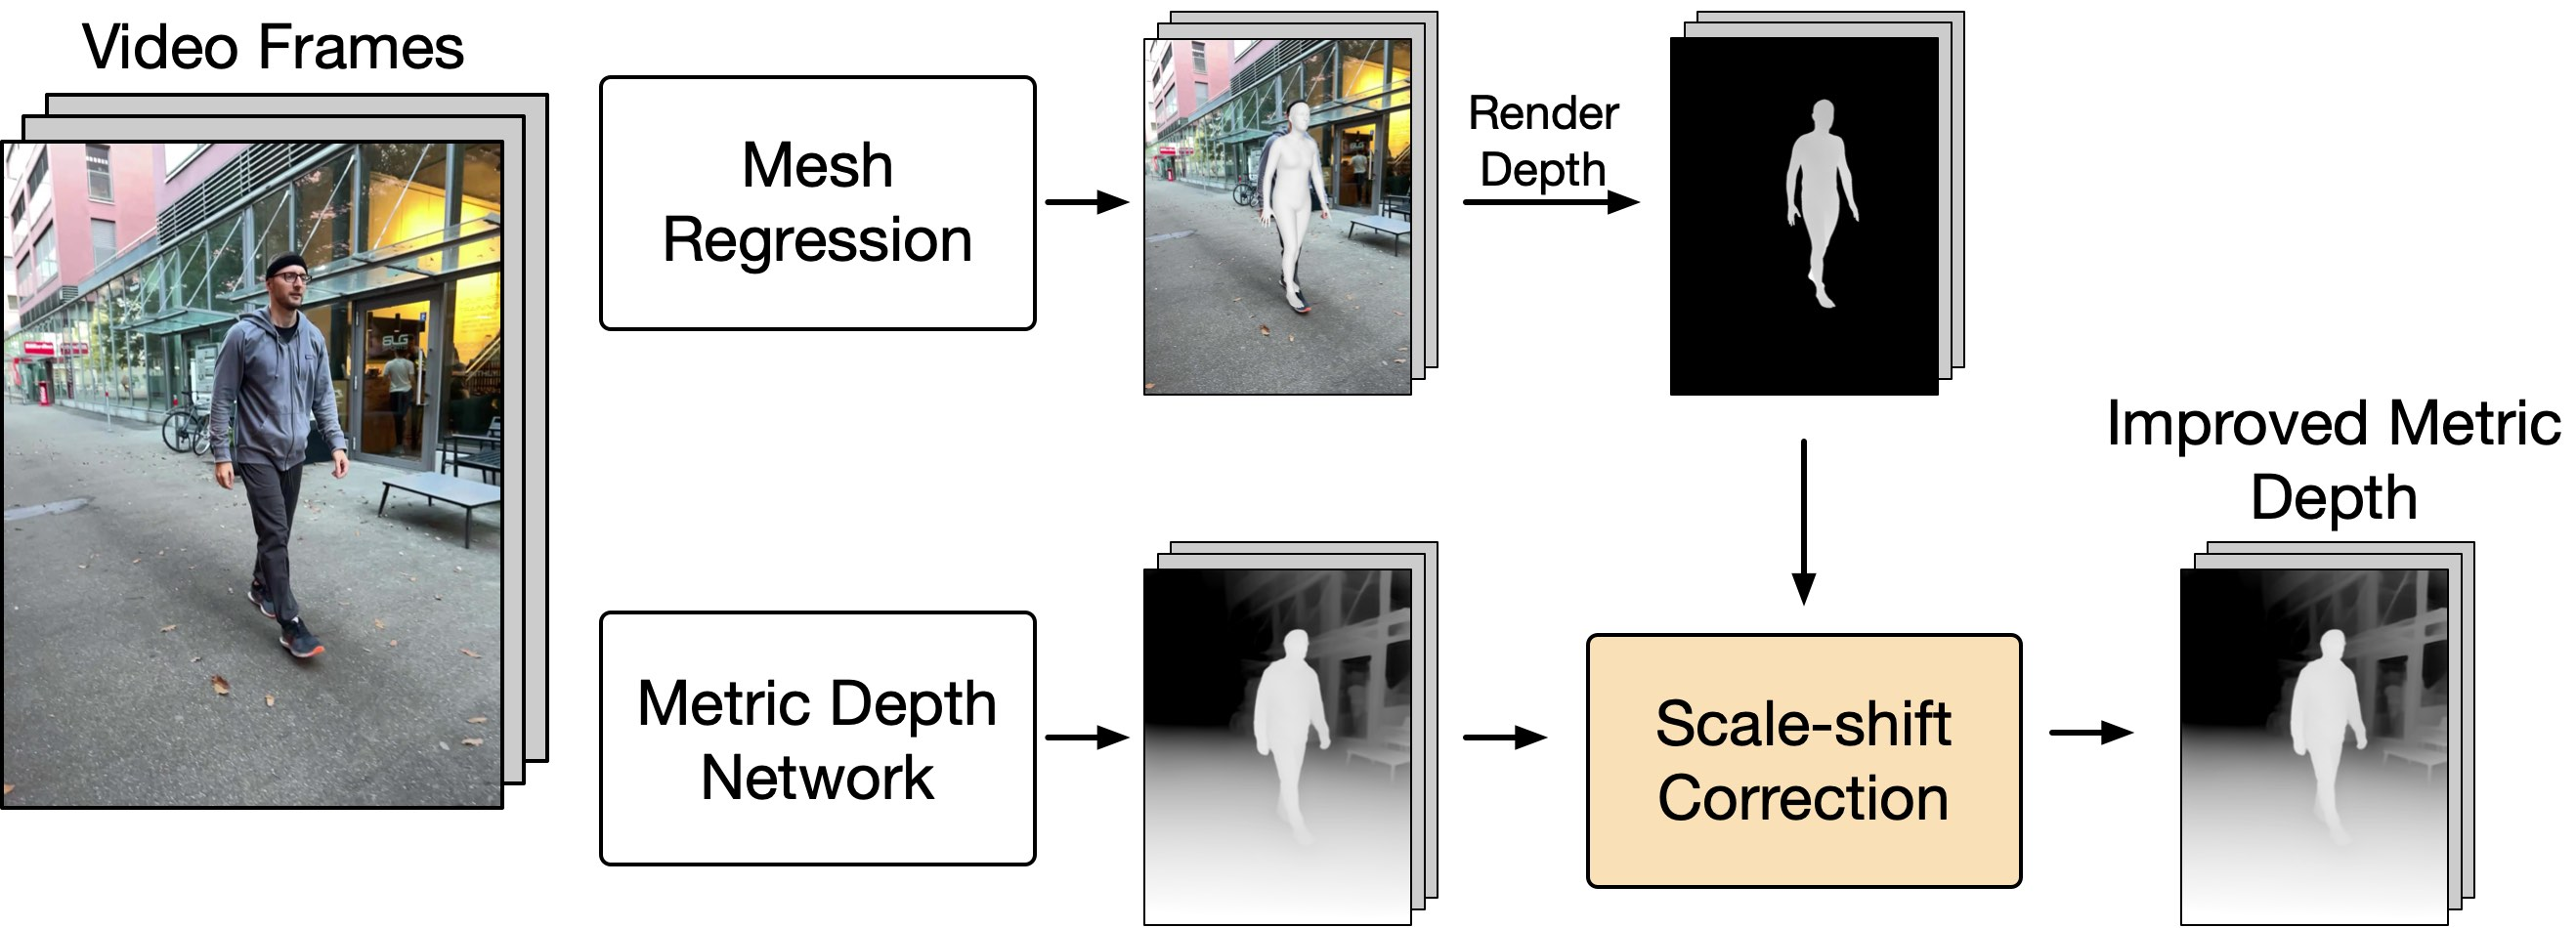}
   \vspace{-1mm}
    \caption{\textbf{Improving depth prediction.} We render depth from SMPL reconstruction, and use this depth map to correct any shift or scale biases in the metric depth prediction. We scale and shift the depth prediction so that its human region would align with the rendered SMPL depth.}
    \vspace{-1mm}
    \label{fig:smpl_depth}
\end{figure*}

\begin{table*}[t!]
% \vspace{-1mm}
\centering
\setlength{\tabcolsep}{3pt}
\resizebox{0.90\textwidth}{!}
{\small{
\begin{tabular}{l?cccc}
\cmidrule{1-5}
& \multicolumn{4}{c}{EMDB 2 (ATE-S)} \\
\cmidrule(lr){2-5}

Scale Estimation using & Short(5) & Medium(10) & Long(10) & Average \\
\cmidrule{1-5}
ZoeDepth & 0.48 & 0.62 & \textbf{0.78} & \textbf{0.66} \\
ZoeDepth + shift correction & 0.37 & \textbf{0.36} & 1.41 & 0.78 \\
ZoeDepth + scale-shift correction & \textbf{0.35} & 0.37 & 1.43 & 0.79 \\
\cmidrule{1-5}
\end{tabular}
}}
\caption{\textbf{Camera scale estimation}. Using SMPL depth rendering to correct scale and shift in depth prediction produces mixed results. 
}
\vspace{-2mm}
\label{tab:scale_smpl}
\end{table*}

We have shown that ZoeDepth prediction is not always accurate. Particularly, there could be shift and scale biases. In such cases, the metric depth prediction can be regarded as affine-invariant depth prediction. If there are objects of known depth in the image, we can use them to correct the shift and scale. Can we use human mesh reconstruction to help correct the biases? Specifically, could we estimate shift and scale variables $s$ and $t$ to correct depth prediction $\hat{D} = s*D + t$?

Figure~\ref{fig:smpl_depth} illustrates this approach. We solve for the scale and shift correction by aligning the human region in the depth prediction to the rendered depth from SMPL reconstruction, through energy minimization similar to the robust optimization in Sec~\ref{sec:3_3} of the main text. We report the quantitative results in Table~\ref{tab:scale_smpl}.  We observe mixed results: it improves scale estimation in some sequences but decreases accuracy in others. Specifically, we observe that it decreases ATE-S (better) by $20\%$ in 10/25 sequences but increases ATE-S (worse) by $20\%$ in 5/25 sequences. The average ATE-S is slightly worse, because worse cases happen to be long sequences, so a small error in scale estimation could lead to a much higher translation error. 

The effectiveness of this approach is also influenced by the accuracy of the mesh reconstruction. If the predicted human shape is more accurate, it will be more effective. Inaccurate shape prediction (e.g., the predicted human being is taller than the ground truth) will produce inaccurate depth rendering.
