# Supplementary material for: TRAM: Global Trajectory and Motion of 3D Humans from in-the-wild Videos
Source: arXiv:2403.17346 source file (2024-09-02)
Supplement: Supplementary file 2 [file supp_b.tex]

\section{Implementation Details}

\begin{figure*}[t!]
\centering
   \includegraphics[width=0.9\textwidth]{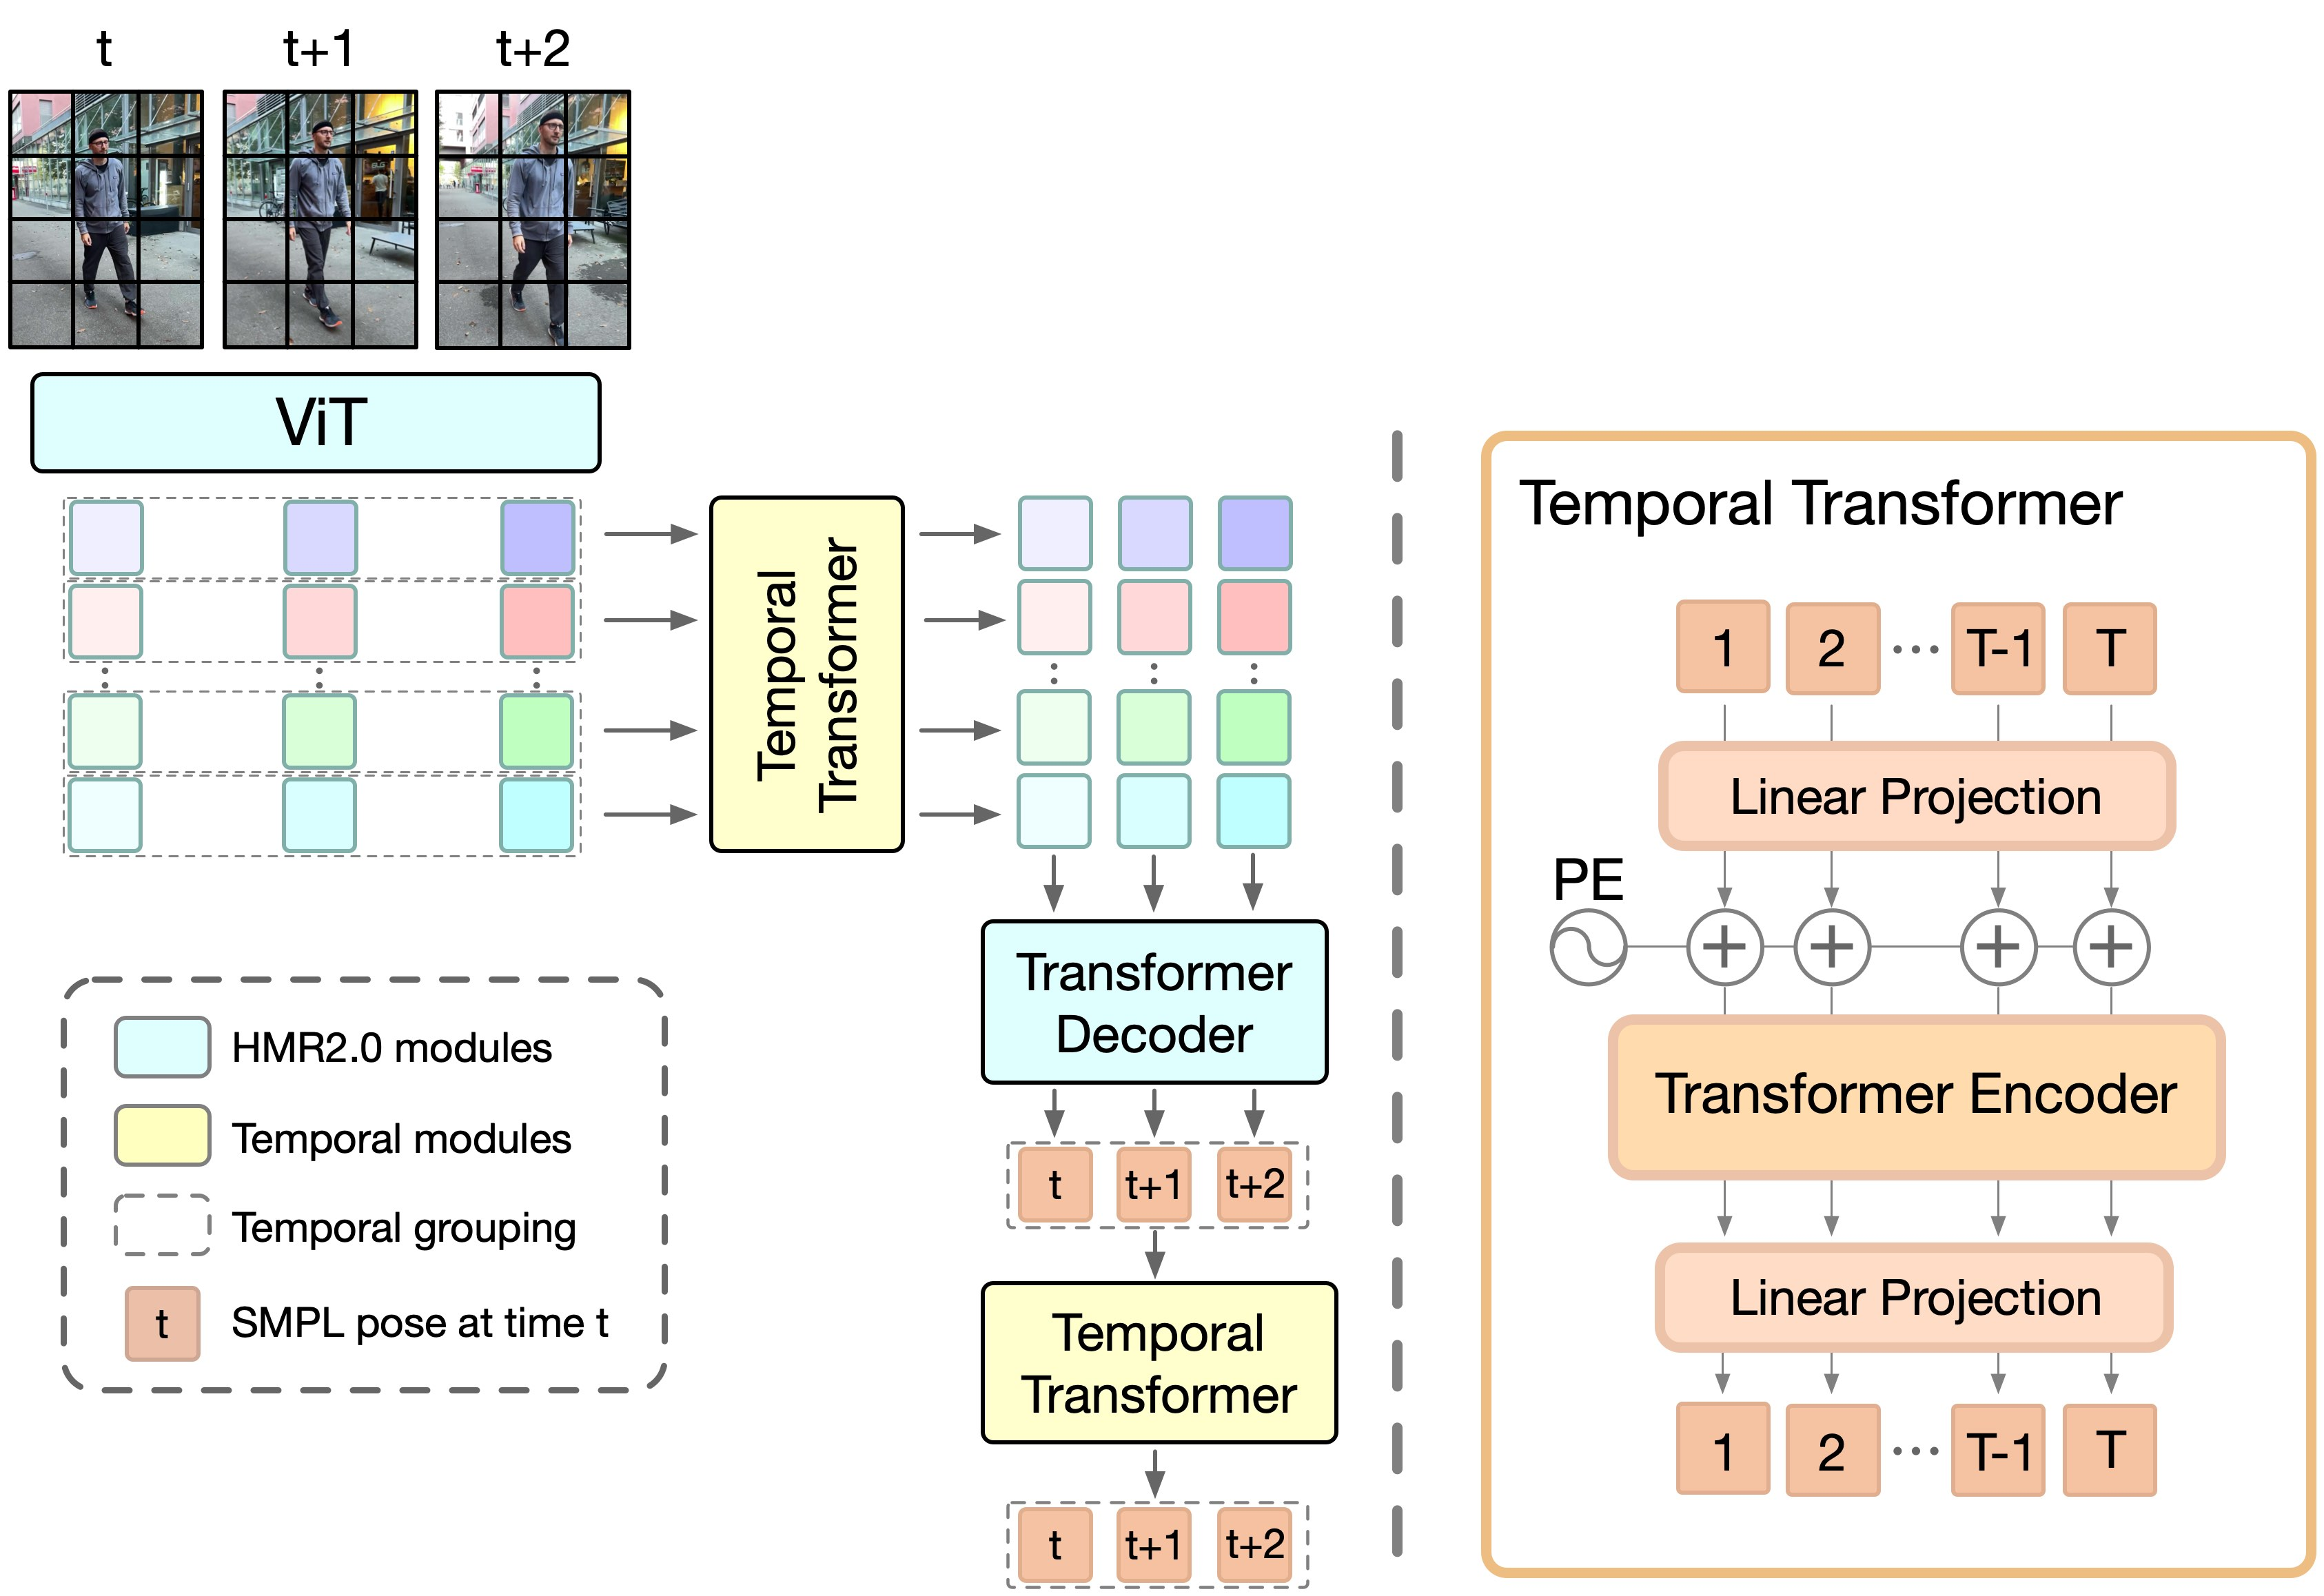}
   \vspace{-1mm}
    \caption{\textbf{Architecture of VIMO.} Left: the detailed architecture of VIMO, with the yellow blocks denoting the new temporal components. Right: the architecture of the two temporal transformers.}
    \vspace{-1mm}
    \label{fig:vimo_detail}
\end{figure*}

\subsection{Architecture}
We show a more detailed view of the VIMO architecture in Figure~\ref{fig:vimo_detail}. VIMO interleaves spatial and temporal modules. Both temporal transformers have 6 layers and 4 multi-head attention. The first temporal transformer (image domain) has an embedding dimension of 512, while the second temporal transformer (motion domain) has an embedding dimension of 384.

\subsection{Datasets}

We use 3DPW, Human3.6M, and BEDLAM to train our video transformer VIMO. We evaluate on 3DPW and EMDB. \textbf{3DPW} is an in-the-wild dataset providing ground truth 3D pose annotations acquired with IMU and videos. 2D and 3D joints are generated from the pose annotation. \textbf{Human3.6M} is an indoor multi-view dataset with 2D and 3D joint annotation. Additionally, we use SMPL recovered using MoSH for this dataset. \textbf{BEDLAM} is a large synthetic dataset rendered with Unreal Engine 5 and SMPL. Therefore, it has the most accurate SMPL pose and shape. \textbf{EMDB} is an in-the-wild dataset with accurate SMPL and trajectory annotations recovered with electromagnetic sensors. 

During training, we sample sequences of 16 frames from the three datasets. There are about 1.3k sequences from 3DPW, 19k from Human3.6M, and 305k from BEDLAM (30fps). So we sample sequences unequally from each dataset to guarantee a good mix of real and synthetic data, with the following ratio: [3DPW: 16.5\%, Human3.6M: 16.5\%, BEDLAM: 67\%].

\subsection{ORB-SLAM2}
We use the open source ORB-SLAM2 implementation released by the authors in \url{https://github.com/raulmur/ORB_SLAM2}. For the masked evaluation, we first process the images in the dataset by setting all pixels within the human masks to a value of 255. We run the entire ORB-SLAM2 pipeline including camera tracking, point reconstruction, and loop closure. We specify our configuration based on the default monocular SLAM parameters for the TUM RGB-D dataset provided in the code and increase the number of features detected at each frame to 4,000. Additionally, because the EMDB videos sometimes demonstrate low contrast with a uniform background,  we slightly lowered the minimum fast feature threshold per image patch (more details in the ORB-SLAM2 configuration documentation). Despite these efforts, we still observed tracking failures due to a fast-moving camera as well as textureless background regions. Compared to ORB-SLAM2, DROID performed better in handling these areas because they do not rely on distinctive sparse features; instead, DROID uses optical flow to guide correspondence, which shares the benefits of low-texture texture handling with direct SLAM methods. For loop closure, we use the bag-of-words vocabulary provided in the official repository.

\subsection{Training}

\textbf{Acceleration.} The training of video models is costly. Because the backbone is often frozen, previous methods pre-compute the features output by the backbone and use them as input to finetune the upper layers (including new components). While this approach reduces forward time, it is impossible to apply data augmentation. To address this issue, we do not pre-compute features but use two other methods: pre-cropping images and half-precision backbone inference. The datasets provide high-resolution images which could take longer to load, crop, and resize. Pre-cropping the images and saving them as crops reduces loading time. Using crops has a different disadvantage: data augmentation such as random rotation and scaling will produce black borders. While it could potentially reduce the effectiveness (it's not clear the extent), it is still better than no augmentation. Secondly, we use half-precision inference for the backbone, which reduces forward
time. Since we do not finetune the backbone, using half-precision will not affect the training. 

\textbf{Data Augmentation.} We apply standard data augmentation including rotation, scaling, horizontal flipping, color jittering, and occlusion. For video model training, all augmentations except occlusion are applied consistently in the same sequence. For example, the same degree of random rotation should be applied for all 16 frames of a sequence. However, each frame has an independent and equal chance of having occlusion augmentation.
