# Supplementary material for: TRAM: Global Trajectory and Motion of 3D Humans from in-the-wild Videos
Source: arXiv:2403.17346 source file (2024-09-02)
Supplement: Supplementary file 3 [file supp_slam.tex]

\begin{table*}[t!]
% \vspace{-1mm}
\centering
\setlength{\tabcolsep}{3pt}
\resizebox{0.90\textwidth}{!}
{\small{
\begin{tabular}{l?cccc}
\cmidrule{1-5}
& \multicolumn{4}{c}{EMDB 2 (ATE-S)} \\
\cmidrule(lr){2-5}

Scale Estimation using & Short(5) & Medium(10) & Long(10) & Average \\
\cmidrule{1-5}
ZoeDepth & 0.48 & 0.62 & \textbf{0.78} & \textbf{0.66} \\
ZoeDepth + shift correction & 0.37 & \textbf{0.36} & 1.41 & 0.78 \\
ZoeDepth + scale-shift correction & \textbf{0.35} & 0.37 & 1.43 & 0.79 \\
\cmidrule{1-5}
\end{tabular}
}}
\caption{\textbf{Camera scale estimation}. Using SMPL depth rendering to correct scale and shift in depth prediction produces mixed results. 
}
\vspace{-2mm}
\label{tab:scale_smpl}
\end{table*}
